# Supplementary material for: Code Generation from Natural Language with Less Prior and More Monolingual Data
Source: arXiv:2101.00259 source file (2021-06-10)
Supplement: Supplementary file 1 [file acl2021_appendix.tex]

%
% File acl2020.tex
%
%% Based on the style files for ACL 2020, which were
%% Based on the style files for ACL 2018, NAACL 2018/19, which were
%% Based on the style files for ACL-2015, with some improvements
%%  taken from the NAACL-2016 style
%% Based on the style files for ACL-2014, which were, in turn,
%% based on ACL-2013, ACL-2012, ACL-2011, ACL-2010, ACL-IJCNLP-2009,
%% EACL-2009, IJCNLP-2008...
%% Based on the style files for EACL 2006 by 
%%e.agirre@ehu.es or Sergi.Balari@uab.es
%% and that of ACL 08 by Joakim Nivre and Noah Smith

\documentclass[11pt,a4paper]{article}
\usepackage[hyperref]{acl2021}
\usepackage{acl2021}
\usepackage{times}
\usepackage{latexsym}

\usepackage{microtype}
\usepackage{amsfonts}
\usepackage{amsmath}
\usepackage{amssymb}
\usepackage{breqn}
\usepackage{graphicx}
\usepackage{tikz}
\usepackage{xspace}
\usepackage{xcolor}
\usepackage{lipsum}
\usepackage{makecell}
\usepackage{tabularx}
\usepackage{listings}
\usepackage{textcomp}
\usepackage{color, colortbl}

%\lstset{language=Python,frame=single,basicstyle=\tiny}
\definecolor{light-gray}{gray}{0.95}
\lstset{language=Python,
    %keywordstyle=\color{blue},
    basicstyle=\tiny\ttfamily\bfseries,
    commentstyle=\color{Green}\ttfamily,
    backgroundcolor=\color{light-gray},
    rulecolor=\color{black},
    aboveskip=-.5\baselineskip,
    belowskip=-2.2em,
    upquote=true,
    showstringspaces=false,
    breaklines=true,
    framesep=0pt,
}
\lstset{escapeinside={<@}{@>}}

\usepackage[shortlabels]{enumitem}

\input{defs}
% This is not strictly necessary, and may be commented out,
% but it will improve the layout of the manuscript,
% and will typically save some space.
\usepackage{microtype}

%\aclfinalcopy % Uncomment this line for the final submission
%\def\aclpaperid{***} %  Enter the acl Paper ID here

%\setlength\titlebox{5cm}
% You can expand the titlebox if you need extra space
% to show all the authors. Please do not make the titlebox
% smaller than 5cm (the original size); we will check this
% in the camera-ready version and ask you to change it back.

\title{Code Generation from Natural Language with \\
 Less Prior and More Monolingual Data}

%% \title{Semantic Parsing with Less Prior Knowledge and More Unlabeled Data}

\author{Sajad Norouzi \\
  Borealis AI\\
  \small \texttt{sajad.norouzi@borealisai.com} \\\And
  Keyi Tang \\
  Borealis AI\\
  \small \texttt{keyi.tang@borealisai.com} \\\And
  Yanshuai Cao \\
  Borealis AI \\
  \small \texttt{yanshuai.cao@borealisai.com} \\}

\date{}

\begin{document}
% \maketitle
% \begin{abstract}
%   \input{abstract}
% \end{abstract}

% \vspace{-0.15cm}
% \section{Introduction}
% \vspace{-0.15cm}

% %\blfootnote{Work in progress}
% \input{intro}

% \section{Previous Work on Semantic Parsing}
% \label{sec:related}
% \input{relatedwork}

% \section{Background and Methodology}
% \input{method}

% \vspace{-0.15cm}
% \section{Experiments}
% \vspace{-0.2cm}
% \input{experiments}

% \section{Conclusion}
% \vspace{-0.15cm}
% \input{conclusion}

\appendix

\onecolumn
\input{appendix}

\bibliography{acl2021}
\bibliographystyle{acl_natbib}

\end{document}
